# Supplementary material for: Spin excitations in optimally P-doped BaFe2(As0.7P0.3)2superconductor
Source: arXiv:1609.01021 source file (2016-09-05)
Supplement: Supplementary file 1 [file Supplementary.pdf]

**Supplementary information on "Spin excitations in optimally P-doped $BaFe_2(As_{0.7}P_{0.3})_2$ superconductor"**

Figure S1 summarizes the basic characteristic of our optimally P-doped superconducting sample. As shown in Fig. S1(a), many samples are aligned using a X-ray Laue machine and glued on thin aluminum plates with hydrogen free glue. The crystallographic directions of the crystals are marked as a, b, and c. Figure S1(b) shows temperature dependence of the resistivity and magnetic susceptibility, revealing a clear superconducting $T_c$ of ~30 K.

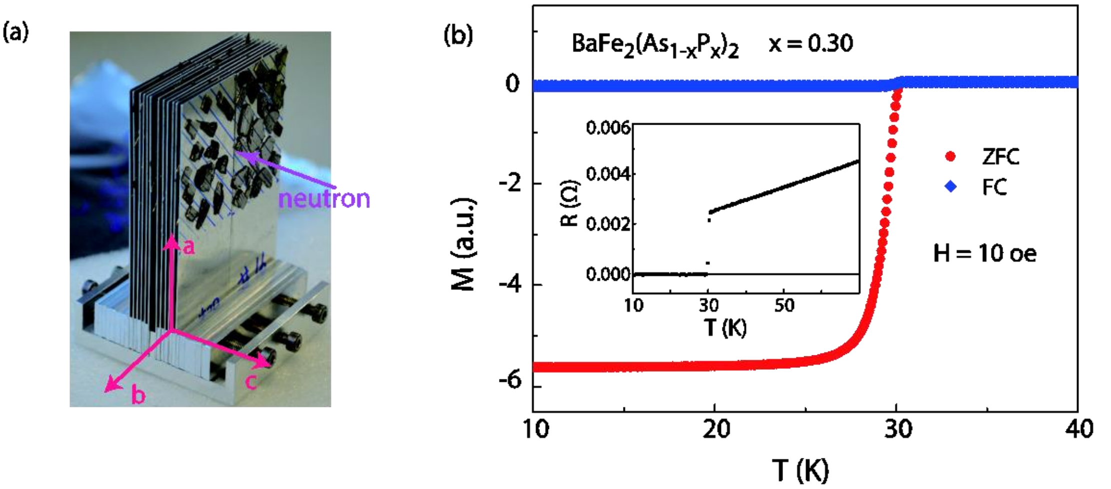


Supplementary Figure S1: (a) The photography of the samples and the setup used in our Time of Flight experiments. (b) Temperature dependence of magnetization under zero-field-cooled and field-cooled for x=0.30 sample with a field of 10 Oe applied perpendicular the c-axis. Inset: Temperature-dependent of resistance.

Figure S2 compares the calculated band structures of $BaFe_2As_2$ and $BaFe_2(As_{0.7}P_{0.3})_2$ used in our DFT+DMFT calculations.

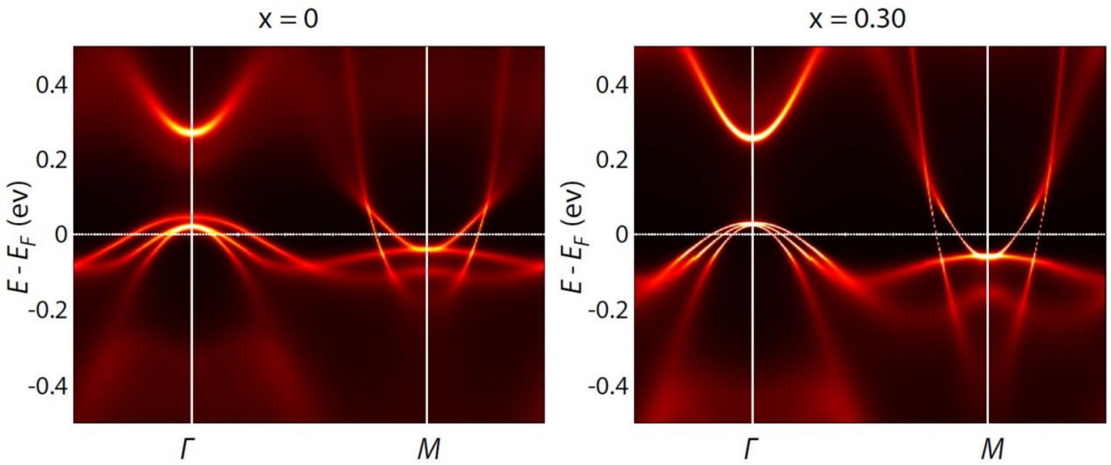

Supplementary Figure S2: comparison of the band structures of x=0 and x=0.30 compounds.

Figure S3 shows cuts of the spin excitations along the [H,0], and [1,K] direction for $BaFe_2(As_{0.7}P_{0.3})_2$.

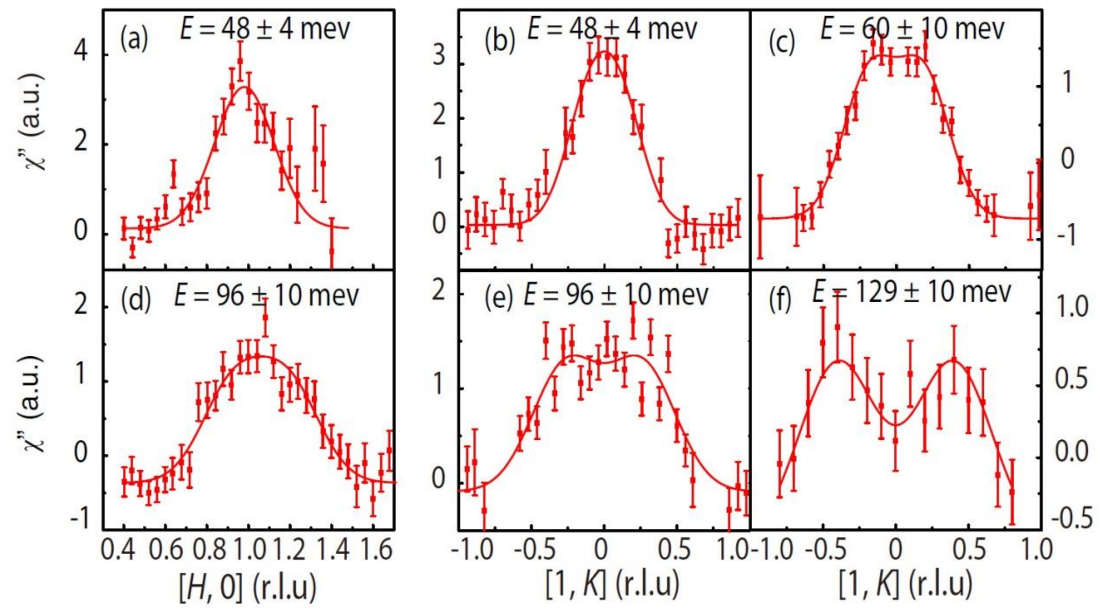


Supplementary Figure S 3: Spin excitation cuts in arbitrary units (a.u.) for $BaFe_2(As_{0.7}P_{0.3})_2$. (a,d): Evolution of spin excitation along the [H, 0] direction, with Ei = 80 mev and 250mev respectively and integrated K = ± 0.1. (b,c,e,f,): Evolution of spin excitations along the [1, K] direction, with integrated H = 1±0.1, (b) is from Ei = 80mev data and (c,e,f) from Ei = 250mev data. The solid lines are from Gaussian fits to the data.

Figure S4 shows cuts of the spin excitations along the [H,0], and [1,K] direction for $BaFe_2As_2$ and $BaFe_2(As_{0.7}P_{0.3})_2$ to test the wave vector evolution of the spin excitations as a function of increasing P-doping. Figure S5 compares high-energy spin waves from $BaFe_2As_2$ and spin excitations from $BaFe_2(As_{0.7}P_{0.3})_2$, and their comparison with spin wave fitting result cuts for $BaFe_2As_2$.

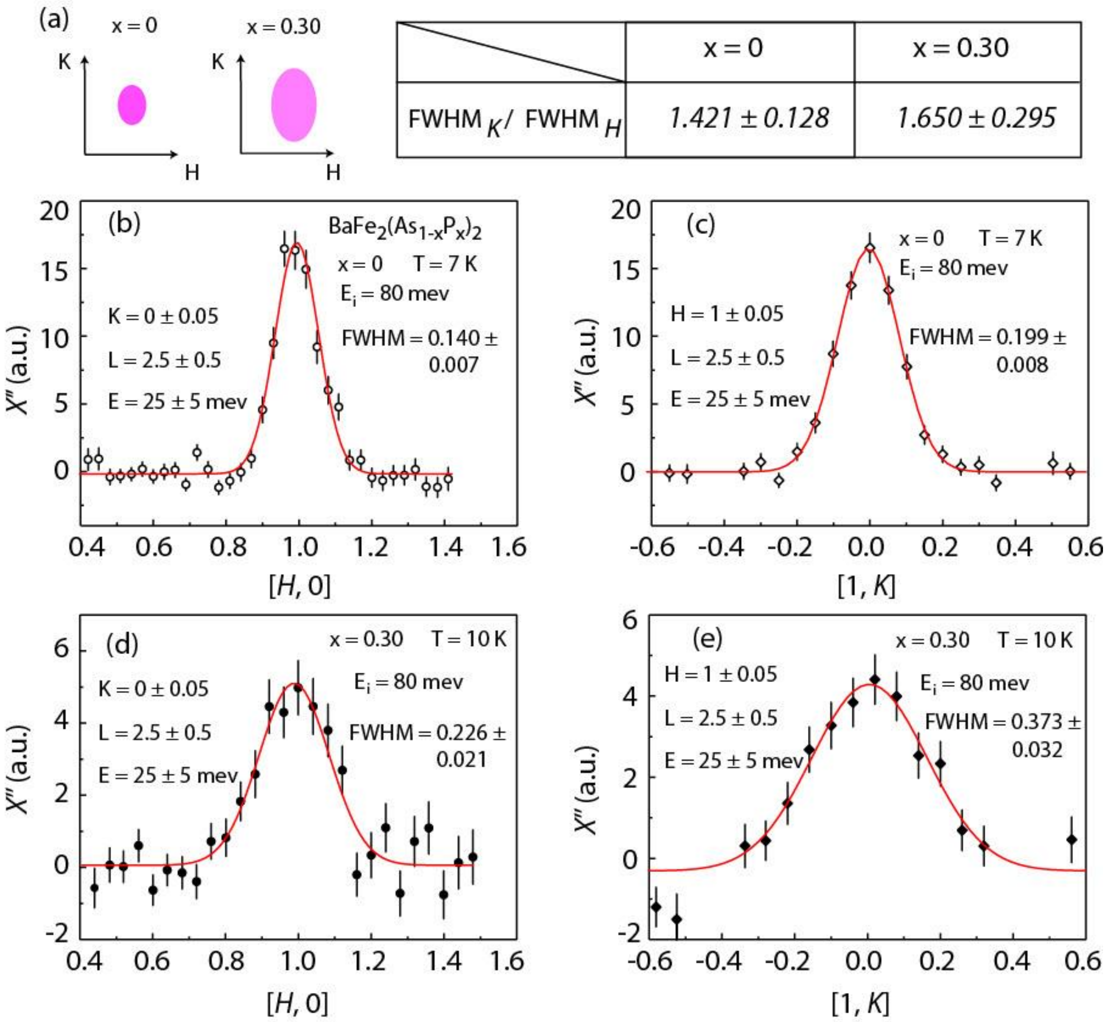


Supplementary Figure S4: Detailed comparison of low energy spin excitation (20mev-30mev) between x=0 and x=0.30 compounds. (a) the schematic shape of spin excitation in a-b plane. (b) (c) Q-cuts along [H, 0] and [1, K] directions for x = 0 compound. (d) (e) Q-cuts for x=0.30 compound. The solid lines are from the Gaussian fits to the data. Table show the ratio of the FWHM from the fits in K and H directions for both compounds. The P doing expands the elliptical low energy spin excitations and is different from the changes upon electron and hole doping.

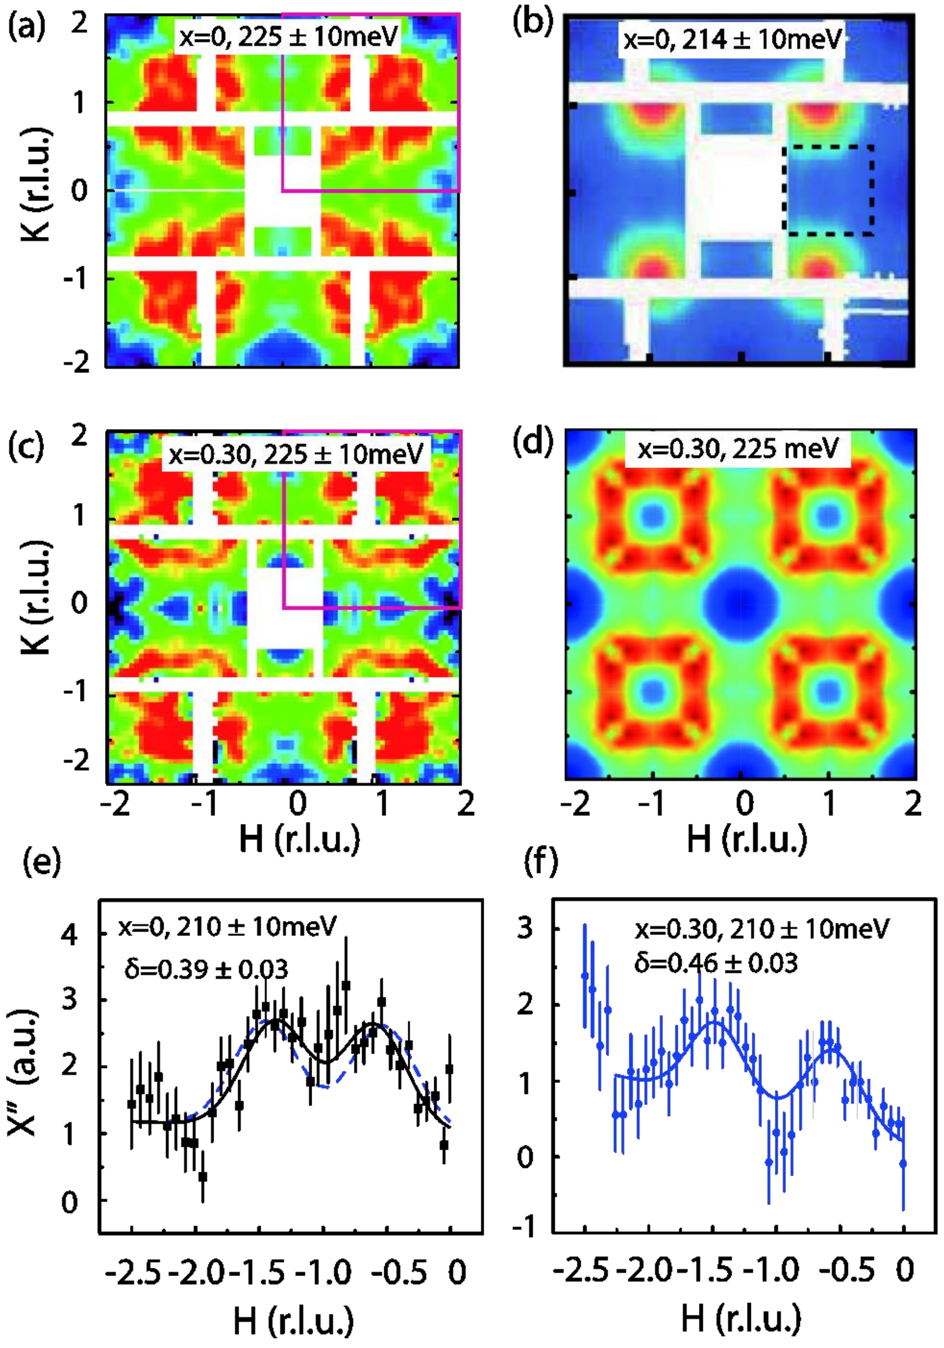


Supplementary Figure S5: (a), (b), (d) are from the figure3 in text. (c) is a similar cut with E = ± 214 meV with the Heisenberg model calculation using anisotropic exchange couplings from fits of the spin wave in $BaFe_2As_2$ [30]. The spin excitations in x=0.30 compound cannot be fitted with a Heisenberg model. (e) and (f) show wave vector cut along the [H,1,0] direction at E= 210 meV for $BaFe_2As_2$ and P-doped samples, respectively. The solid lines in (e) and (f) are fits with two Gaussians on a sloped background symmetrically displaced from (1,1) with a incommensurability distance $\delta$ for P-doped and pure $BaFe_2As_2$, respectively. The incommensurability $\delta$ is clearly larger in the P-doped case, suggesting the scattering has not yet reached zone boundary at this energy. The dashed line in (e) is the fits for P-doped sample.

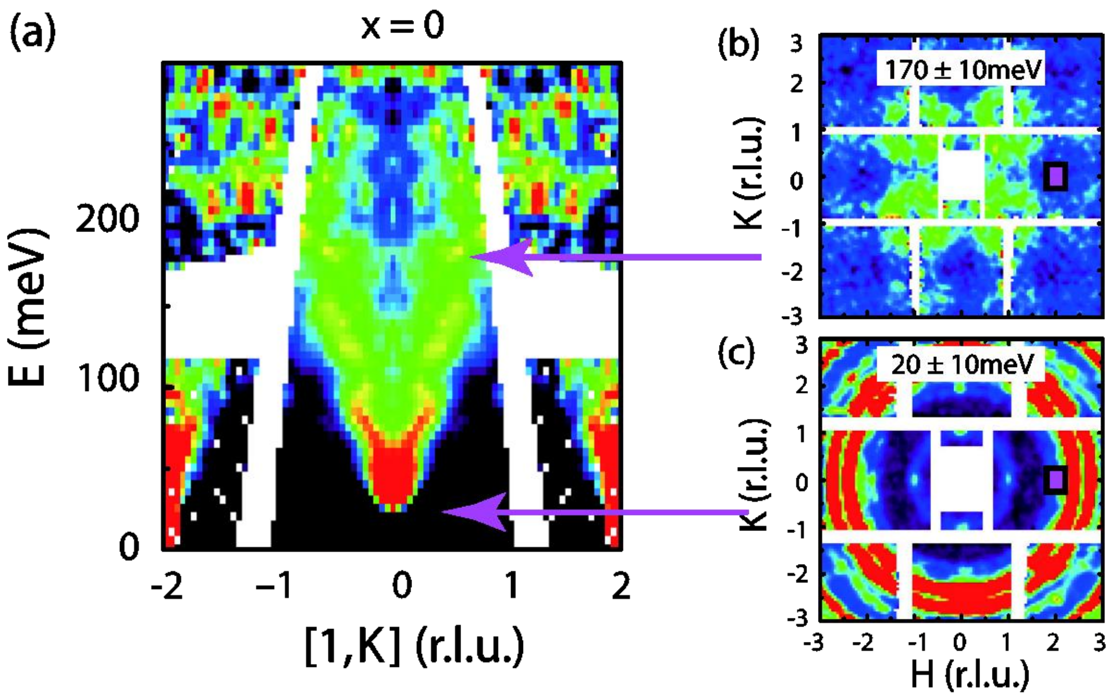


Supplementary Figure S6. Summaries of the background subtraction procedure for the Ei = 450 meV data. Fig. (a) is the spin excitation dispersion from background subtracted data of $BaFe_2As_2$. (b, c) show the raw data at E=20 meV and 170 meV. In the whole energy range, we choose the area 1.8<H<2.2 and -2.5<K<2.5 [purple area in (b, c)] to be the background. While this procedure is reasonable for high energy spin excitations as shown in (b), the low-energy background is over estimated, revealing negative signal in (a). However, such procedure does not affect the overall dispersion of the system. To estimate the background scattering in low energy spin excitations, we will choose lower Ei data and area between magnetic signals to be the background scattering.

Table S1 summarizes our efforts in estimating the magnetic contributions to the superconducting condensation energy following the procedures discussed in [27].

Supplementary Table S1:

| *E* | $\sigma_{x,s}$ | $\sigma_{y,s}$ | $A_s$ | $\sigma_{x,n}$ | $\sigma_{y,n}$ | $A_n$ |
|---|---|---|---|---|---|---|
| 3 | 0 | 0 | 0 | 0.054 | 0.074 | 6.0 |
| 5 | 0.04 | 0.049 | 8.1 | 0.051 | 0.08 | 9.2 |
| 7 | 0.046 | 0.062 | 15.0 | 0.064 | 0.091 | 8.0 |
| 9 | 0.06 | 0.077 | 19.1 | 0.092 | 0.1 | 6.8 |
| 10 | 0.066 | 0.086 | 17.8 | 0.079 | 0.104 | 5.9 |
| 11 | 0.063 | 0.096 | 17.4 | 0.086 | 0.089 | 5.2 |
| 13 | 0.075 | 0.103 | 13.4 | 0.09 | 0.104 | 3.8 |
| 16 | 0.089 | 0.13 | 8.5 | 0.056 | 0.121 | 5.0 |
| 20 | 0.092 | 0.133 | 5.4 | 0.059 | 0.152 | 3.6 |

The fitting parameters of low energy spin excitations in $BaFe_2(As_{0.7}P_{0.3})_2$.

The magnetic exchange coupling changes are:

$\langle S_i \cdot S_{i+x} \rangle_s - \langle S_i \cdot S_{i+x} \rangle_n = -0.0023$, $\langle S_i \cdot S_{i+y} \rangle_s - \langle S_i \cdot S_{i+y} \rangle_n = 0.0022$,
$\langle S_i \cdot S_{i+x+y} \rangle_s - \langle S_i \cdot S_{i+x+y} \rangle_n = \langle S_i \cdot S_{i+x-y} \rangle_s - \langle S_i \cdot S_{i+x-y} \rangle_n = -0.0022$.
The magnetic exchange coupling constants in an anisotropic model are estimated to be $J_{1a}S$ = 65.1 meV, $J_{1b}S$ = -10.1 meV, $J_2S$ = 15.0 meV, which are 10% larger that of $BaFe_2As_2$. Hence the exchange energy change is -0.48mev/Fe.
The condensation energy $U_c$ for optimally doped $BaFe_2(As_{0.7}P_{0.3})_2$ can be calculated to be $U_c$ = -5.5 J/mol = -0.03meV/Fe from the specific heat data of Ref. [49]. Therefore, the changes in magnetic excitation energy due to the formation of the resonance is much larger than the superconducting condensation energy.
